# Supplementary material for: Chiral interactions up to next-to-next-to-next-to-leading order and nuclear saturation
Source: arXiv:1710.08220 ancillary file (2019-02-02)
Supplement: Supplementary file 1 [file supplemental_material.pdf]

# Supplemental Material for
# "Chiral interactions up to next-to-next-to-next-to-leading order and nuclear saturation"

C. Drischler,[1,2,*] K. Hebeler,[1,2,†] and A. Schwenk[1,2,3,‡]

[1] *Institut für Kernphysik, Technische Universität Darmstadt, 64289 Darmstadt, Germany*
[2] *ExtreMe Matter Institute EMMI, GSI Helmholtzzentrum für Schwerionenforschung GmbH, 64291 Darmstadt, Germany*
[3] *Max-Planck-Institut für Kernphysik, Saupfercheckweg 1, 69117 Heidelberg, Germany*

## FIT TO $^3$H BINDING ENERGY

Figure 1 shows the constraint on the 3N couplings $c_D$ and $c_E$ by requiring that the corresponding NN and 3N interactions reproduce the $^3$H binding energy. The details on the interactions are given in the main text.

## BENCHMARKS AT THIRD ORDER

Table I compares our symmetric-matter results based on the N$^3$LO NN potential of Ref. [2] at third order to the partial-wave-based calculations by Holt *et al.* [3] at three densities. The particle-particle and hole-hole contributions have also been successfully benchmarked against our previous calculations [4–6]. The small deviation for the particle-hole contribution likely originates from the different partial-wave truncations, which have less of an impact on the other channels. We therefore also benchmarked against the semianalytic calculations in Ref. [3], which we reproduce with high accuracy, including the third-order particle-hole term of the ground-state energy of the dilute Fermi gas. A comparison at the normal-ordered two-body level with 3N contributions is unfortunately not straightforward because of the approximations involved in the 3N regulator in Ref. [3]. In addition, we have benchmarked the residual 3N contributions at second order in neutron and symmetric matter with semianalytic calculations at N$^2$LO by Dyhdalo *et al.* [7] for all $c_1$, $c_3$, $c_4$, $c_D$, and $c_E$ topologies.

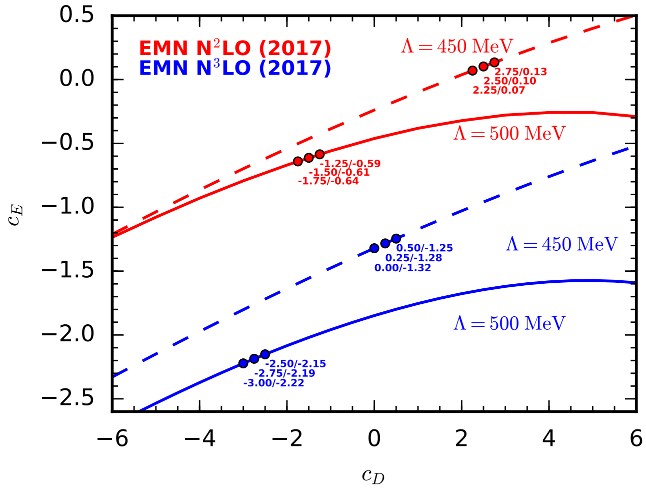


FIG. 1. Three-nucleon couplings $c_D$ and $c_E$ that reproduce the $^3$H binding energy using the EMN NN potentials of Ref. [1] with $\Lambda = 450$ MeV (dashed) and $\Lambda = 500$ MeV (solid line) at N$^2$LO (red) and N$^3$LO (blue) combined with consistent 3N interactions at these orders using $\Lambda = \Lambda_{\mathrm{NN,3N}}$. The points on each line correspond to the fits to the empirical saturation region (see the diamonds in Fig. 3 of the main text), while the annotated numbers give the corresponding values of $c_D/c_E$.

TABLE I. Comparison to partial-wave-based calculations at third order by Holt *et al.* [3] in symmetric nuclear matter. Densities are given in fm$^{-3}$, while energies are in MeV. A free spectrum is used. The abbreviations hh, pp, and ph stand for hole-hole, particle-particle, and particle-hole contribution, respectively.

| | density | Holt *et al.* | this work |
|---|---|---|---|
| third order hh | 0.16 | −0.47 | −0.46 |
| third order hh | 0.21 | −0.56 | −0.54 |
| third order pp | 0.16 | +1.03 | +1.02 |
| third order pp | 0.21 | +1.75 | +1.75 |
| third order ph | 0.17 | −1.93 | −1.89 |
| third order ph | 0.21 | −2.57 | −2.51 |

## ENERGY PER PARTICLE AT LEADING AND NEXT-TO-LEADING ORDER

Figure 2 shows the energy per particle in neutron and symmetric matter based on the EMN potentials at LO and NLO for the cutoffs $\Lambda = 450$ and 500 MeV. Due to cancellations of different contributions in neutron matter, the two cutoffs lead to very similar results (so that the two lines are on top of each other). Note that 3N forces are not present in the chiral expansion at these orders.

## MANY-BODY CONVERGENCE

Table II gives more details on the MBPT convergence at fixed densities.

TABLE II. Contributions to the energy per particle at several densities in symmetric nuclear matter at consecutive orders in MBPT based on the Hebeler+ [4] interaction with $\lambda/\Lambda_{3N} = 1.8/2.0\ \mathrm{fm}^{-1}$ and the N$^2$LO and N$^3$LO interactions of this work with $\Lambda/c_D$ [for the central $c_D$ fit value (black diamonds) in Fig. 3 of the main text]. All energies are in MeV.

| chiral order | $\Lambda/c_D$ | density | | Hartree-Fock | | second order | | | third order | | fourth order |
|---|---|---|---|---|---|---|---|---|---|---|---|
| | | in fm$^{-3}$ | kinetic | NN-only | 3N-only | NN-only | NN+3N | 3N res. | NN-only | NN+3N | NN-only |
| N$^3$LO/N$^2$LO | $\lambda/\Lambda_{3N} = 1.8/2.0\,\mathrm{fm}^{-1}$ | 0.08 | 13.93 | −24.97 | 1.79 | −2.93 | −2.95 | −0.08 | −0.23 | −0.11 | −0.29 |
| | | 0.12 | 18.25 | −34.85 | 4.21 | −2.59 | −2.71 | −0.10 | −0.04 | −0.05 | −0.23 |
| | | 0.16 | 22.11 | −43.80 | 7.61 | −2.30 | −2.54 | −0.10 | 0.04 | −0.10 | −0.20 |
| | | 0.20 | 25.65 | −52.02 | 11.92 | −2.10 | −2.44 | −0.08 | 0.08 | −0.23 | −0.18 |
| N$^2$LO | 450/+2.50 | 0.08 | 13.93 | −19.54 | 2.63 | −6.14 | −8.02 | −0.25 | −0.19 | −0.08 | 0.14 |
| | | 0.12 | 18.25 | −27.24 | 6.47 | −6.34 | −10.60 | −0.36 | 0.11 | −0.88 | 0.15 |
| | | 0.16 | 22.11 | −34.16 | 12.10 | −6.23 | −13.38 | −0.42 | 0.23 | −2.08 | 0.07 |
| | | 0.20 | 25.65 | −40.45 | 19.53 | −6.08 | −16.25 | −0.43 | 0.28 | −3.16 | 0.00 |
| | 500/−1.50 | 0.08 | 13.93 | −18.17 | 2.45 | −7.49 | −8.86 | −0.31 | −0.13 | 0.22 | 0.25 |
| | | 0.12 | 18.25 | −25.28 | 5.87 | −8.27 | −11.59 | −0.51 | 0.17 | −0.12 | 0.38 |
| | | 0.16 | 22.11 | −31.64 | 10.85 | −8.61 | −14.49 | −0.66 | 0.28 | −0.77 | 0.32 |
| | | 0.20 | 25.65 | −37.38 | 17.39 | −8.75 | −17.60 | −0.76 | 0.31 | −1.17 | 0.20 |
| N$^3$LO | 450/+0.25 | 0.08 | 13.93 | −18.37 | 2.79 | −7.47 | −9.02 | −0.16 | −0.35 | −0.51 | 0.49 |
| | | 0.12 | 18.25 | −25.76 | 6.59 | −8.37 | −11.82 | −0.26 | 0.02 | −1.18 | 0.65 |
| | | 0.16 | 22.11 | −32.54 | 12.02 | −8.84 | −14.52 | −0.32 | 0.23 | −2.28 | 0.61 |
| | | 0.20 | 25.65 | −38.84 | 19.03 | −9.17 | −17.15 | −0.35 | 0.36 | −3.43 | 0.49 |
| | 500/−2.75 | 0.08 | 13.93 | −18.01 | 2.68 | −7.98 | −9.07 | −0.31 | −0.45 | −0.36 | 0.36 |
| | | 0.12 | 18.25 | −24.97 | 6.13 | −9.44 | −12.02 | −0.58 | −0.23 | −0.61 | 0.58 |
| | | 0.16 | 22.11 | −31.19 | 10.93 | −10.56 | −14.98 | −0.83 | −0.16 | −1.05 | 0.65 |
| | | 0.20 | 25.65 | −36.85 | 17.03 | −11.57 | −18.02 | −1.04 | −0.16 | −1.40 | 0.65 |

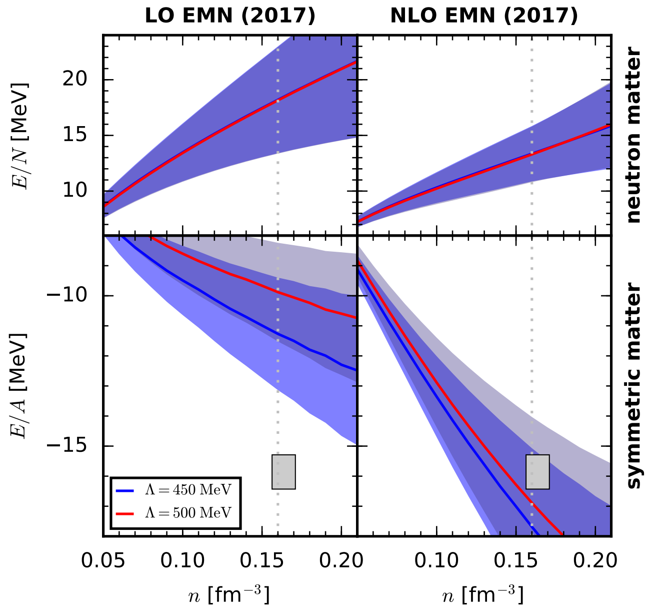


FIG. 2. Energy per particle in neutron matter (top row) and symmetric nuclear matter (bottom row) based on chiral interactions at LO (first column) and NLO (second column). The blue ($\Lambda = 450$ MeV) and gray ($\Lambda = 500$ MeV) bands estimate the theoretical uncertainty following Ref. [8].

* Email: christian.drischler@physik.tu-darmstadt.de
† Email: kai.hebeler@physik.tu-darmstadt.de
‡ Email: schwenk@physik.tu-darmstadt.de

[1] D. R. Entem, R. Machleidt, and Y. Nosyk, Phys. Rev. C **96**, 024004 (2017).
[2] D. R. Entem and R. Machleidt, Phys. Rev. C **68**, 041001(R) (2003).
[3] J. W. Holt and N. Kaiser, Phys. Rev. C **95**, 034326 (2017).
[4] K. Hebeler, S. K. Bogner, R. J. Furnstahl, A. Nogga, and A. Schwenk, Phys. Rev. C **83**, 031301(R) (2011).
[5] C. Drischler, K. Hebeler, and A. Schwenk, Phys. Rev. C **93**, 054314 (2016).
[6] C. Drischler, A. Carbone, K. Hebeler, and A. Schwenk, Phys. Rev. C **94**, 054307 (2016).
[7] A. Dyhdalo, R. J. Furnstahl, K. Hebeler, and I. Tews, Phys. Rev. C **94**, 034001 (2016).
[8] E. Epelbaum, H. Krebs, and U.-G. Meißner, Eur. Phys. J. A **51**, 53 (2015).
